# Supplementary material for: Generative 3D Part Assembly via Part-Whole-Hierarchy Message Passing
Source: arXiv:2402.17464 source file (2024-03-27)
Supplement: Supplementary file 1 [file X_suppl.tex]

\clearpage
\setcounter{page}{1}
\maketitlesupplementary

\section{Experimental Details}

\subsection{Training details}

Our model is implemented with Pytorch, which is trained for around 1000 epochs to converge. The initial learning rate is set as 0.0001, and we employ AdamW to optimize the whole model. We treat the poses of super-parts as latent variables and only train the model with ground-truth part poses as supervision. We train our model on eight GeForce RTX 3090 GPUs with a batch size of 64. The dimension of the random Gaussian noise was set to 80. The number of multi-head self-attention layers in the super-part encoder and part encoder was set to 2 and 6, respectively.  

We obtain the part-whole hierarchy by partitioning the parts into geometrically-equivalent part clusters, where each cluster serves as a super part. Following \cite{zhan2020generative,zhang20223d}, in order to identify geometrically-equivalent parts, we begin by excluding parts whose Axis-Aligned-Bounding-Box dimensions differ by more than 0.1. Next, we further refine the selection by eliminating pairwise parts with a Chamfer distance below an empirically determined threshold of 0.2.

\subsection{Evaluation Metrics}

We now provide more details of the evaluation metrics.

\subsubsection{Part Assembly Quality Evaluation}
Following \cite{zhan2020generative,narayan2022rgl,zhang20223d}, we use \textit{shape Chamfer distance} (SCD), \textit{part accuracy} (PA) and \textit{connectivity accuracy} (CA) to measure the quality of assembled shapes. \textit{Shape Chamfer distance} is defined in Equation \eqref{eq:CD} and Equation \eqref{eq:SCD}. The definitions of the remaining terms are provided below.

\textbf{Part Accuracy} This metric measures the percentage of matched parts within a centain Chamfer distance threshold, formally,
\begin{equation}
    \text{PA}\left(\tau_p \right)=\frac{1}{N}\sum\limits_{i=1}^N\mathbbm{1} \bigg(d_c\big( \mathbf{T}_i\left(\mathbf{P}_i \right),\mathbf{T}_i^{\ast}\left(\mathbf{P}_i \right) \big)< \tau_{p} \bigg),
\end{equation}
where $\mathbbm{1}$ represents the indicator function. $\mathbf{T}_i\left(\mathbf{P}_i \right)$ and $\mathbf{T}_i^{\ast}\left(\mathbf{P}_i \right)$ are $SE(3)$ transformed parts and ground-truth parts, respectively.

\textbf{Connectivity Accuracy}
Similar to previous works, we utilize connectivity accuracy to measure the quality of connections between adjacent parts. For each connected part pair $\left\langle 
\mathbf{P}_i, \mathbf{P}_j \right\rangle$, the contact point $c_{ij}^{\ast}$ is defined as a point on $\mathbf{P}_i$ that is closest to $\mathbf{P}_j$, so does $c_{ji}^{\ast}$. The contact-point pair $\left\{c_{ij}^{\ast}, c_{ji}^{\ast} \right\}$ is transformed into part canonical space as $\left\{c_{ij}, c_{ji} \right\}$. Then the connectivity accuracy is calculated as:
\begin{equation}
    \text{CA}\left(\tau_c \right) = \frac{1}{\left| \mathcal{C} \right|} \sum\limits_{\left\{c_{ij}, c_{ji} \right\}\in \mathcal{C}} \mathbbm{1} \bigg(\| \mathbf{T}_i \left(c_{ij} \right)-\mathbf{T}_j\left(c_{ji} \right) \|_2^2 < \tau_{c} \bigg),
\end{equation}
where $\mathcal{C}$ denotes the set of all possible contact point pairs $\left\{c_{ij}, c_{ji}\right\}$. 

\textbf{Mean Accuracy}
The calculation of PA and CA depends on the Chamfer distance threshold $\tau_{p}$ and $\tau_{c}$ for judging whether the assembly is accurate. In order to provide a more comprehensive evaluation of the performance of the model, we also average the results under multiple Chamfer distance thresholds to get \textit{mean part accuracy} (mPA) and \textit{mean connectivity accuracy} (mCA), formally, 
\begin{equation}\label{eq:mpa_mca}
    \text{mPA} = \frac{1}{T_{p}} \sum\limits_{\tau_{p}\in T_{p}}\text{PA}\left(\tau_p \right), \qquad
    \text{mCA} = \frac{1}{T_{c}} \sum\limits_{\tau_{c}\in T_{c}}\text{CA}\left(\tau_c \right). 
\end{equation}

In our experiments, $T_{p}$ and $T_{c}$ are set to $\left\{0.01, 0.02, 0.03, 0.04, 0.05  \right\}$. We report all the results to comprehensively evaluate our model's ability to accurately assemble part point clouds.

\subsubsection{Generative Part Assembly Diversity Evaluation}
In addition to the quality of assembly, the diversity of assembly plays a pivotal role in the generative 3D part assembly task. To compare the diversity of assembled parts with reasonable shapes, we provide both qualitative and quantitative evaluation on different assembly algorithms. 
Following \cite{cheng2023score}, the two quantitative evaluation metrics including the Quality-Diversity Score (QDS) and the Weighted Quality-Diversity Score (WQDS) are defined as follows.

\textbf{QDS} 
Diversity Score (DS)~\cite{mo2020pt2pc,shu20193d} evaluates the diversity of the results: The formula of DS is $\text{DS}=\frac{1}{N^2}\sum\limits_{i,j=1}^N(\text{Dist}(\mathbf{P}_i^{\ast}, \mathbf{P}_j^{\ast}))$, where $\mathbf{P}_i^{\ast}$ and $\mathbf{P}_j^{\ast}$ represent any two assembled shapes. Based on DS, we add constraints to the comparison pair, which not only test the diversity among all transformed shapes but also consider the quality of these transformed shapes. The formula of QDS is
% \begin{equation}
\begin{align}
    \text{QDS}=\frac{1}{N^2}\sum\limits_{i,j=1}^N[\text{Dist}(\mathbf{P}_i^{\ast}, \mathbf{P}_j^{\ast})\cdot \nonumber\\
    \mathbbm{1} (\text{CA}(\mathbf{P}_i^{\ast}>\tau_q))\cdot
    \mathbbm{1} (\text{CA}(\mathbf{P}_j^{\ast}>\tau_q))]. 
    \label{eq:QDS}
\end{align}
% \end{equation}
Following \cite{cheng2023score}, we apply $\text{SCD}$ as the distance metric. The value of $\tau_q$ is set to 0.5 in QDS and WQDS.

\textbf{WQDS} We further add the weight defined by $\text{CA}$ as follows:
\begin{gather}
    \text{WQDS}=\frac{1}{N^2}\sum\limits_{i,j=1}^N[\text{Dist}(\mathbf{P}_i^{\ast}, \mathbf{P}_j^{\ast})\cdot
    \mathbbm{1} (\text{CA}(\mathbf{P}_i^{\ast}>\tau_q))\cdot \nonumber\\ \mathbbm{1} (\text{CA}(\mathbf{P}_j^{\ast}>\tau_q)) \cdot \text{CA}(\mathbf{P}_i) \cdot \text{CA}(\mathbf{P}_j)]. 
    \label{eq:WQDS}
\end{gather}

As previously mentioned, $\text{CA}$ evaluates the connectivity accuracy of the algorithms. The criteria for both metrics imply that the pair contributes to the diversity value only if both assembled shapes exhibit sufficiently high connectivity accuracy. In essence, both assembled shapes should demonstrate a high-quality connection between each pair of parts. These two novel metrics, QDS and WQDS, align with the demands of our tasks, specifically in evaluating the diversity among adequately assembled pairs.

\begin{table}  
  \centering
  \caption{Ablation study on the depth of the part encoder.}
  \resizebox{0.65\columnwidth}{!}{%
  \begin{tabular}{lc|ccc}
    \toprule
    & layers &  SCD$\downarrow$ & PA$\uparrow$ & CA$\uparrow$ \\
    \midrule
    & 2 & 0.0044 & 56.32 & 40.86 \\
    \midrule
    & 4 & 0.0035 & 61.28 & 55.67 \\
    \midrule
    & 6 & \textbf{0.0028}  & \textbf{64.83} & \textbf{58.45} \\
    \midrule
    & 8 & 0.0030 & 63.26 & 57.39 \\
    \bottomrule
  \end{tabular}
  }
  \label{tab:ablationdepth}  
\end{table}

\begin{table}
  \centering
  \caption{Ablation study on the depth of the super-part encoder.}
  \resizebox{0.65\columnwidth}{!}{%
  \begin{tabular}{lc|ccc}
    \toprule
    & layers &  SCD$\downarrow$ & PA$\uparrow$ & CA$\uparrow$ \\
    \midrule
    & 2 & \textbf{0.0028}  & \textbf{64.83} & \textbf{58.45} \\
    \midrule
    & 4 & 0.0029 & 63.49 & 57.62\\
    \midrule
    & 6 & 0.0031 & 63.00 & 56.93 \\
    \midrule
    & 8 & 0.0034 & 62.12 & 55.82 \\
    \bottomrule
  \end{tabular}
  }
  \label{tab:ablationsuperpartdepth}  
\end{table}

\section{Additional qualitative results}
\label{sec:aqr}
We demonstrate additional visual results predicted by our part-whole hierarchy message passing network compared with other methods in Figure \ref{fig:aqr} and Figure \ref{fig:aqr2}.

\section{Additional ablation studies}
\label{sec:aaam}

% \begin{table}
% \begin{minipage}[t]{0.48\linewidth}
% \input{tables/ablationhierarchy}
% \end{minipage}
% \hfill
% \begin{minipage}[t]{0.48\linewidth}
% \input{tables/ablationloss}
% \end{minipage}
% \end{table}

In this section, we explore the significance of multi-head self-attention relationship learning between parts and super-parts by manipulating the number of layers in the part encoder and super-part encoder, respectively. We show the results under a certain Chamfer distance threshold 0.01 on the largest category of  PartNet dataset, \ie, tables. In Table \ref{tab:ablationdepth}, the performance shows a consistent improvement as the number of part encoder layers increases and reaches a plateau at the sixth encoder layer. From Table \ref{tab:ablationsuperpartdepth}, we observe that the performance gradually decreases as the number of super-part encoder layers increases from two. This indicates that learning the super-part relation is comparatively easier than learning the part relation, suggesting that an excessively complex super-part encoder is unnecessary.

\section{Failure cases and future work}
\label{sec:fcfw}
In Figure \ref{fig:fcfw}, We show some cases where our model fails to assemble shapes effectively. In case (a), we have a chair with two disconnected components. Our model produces confusing assembly results, as all parts are geometrically dissimilar and each part is treated as a super-part, failing to take advantage of part-whole hierarchies. In case (b), the pink armrest and the green backrest are geometrically similar and considered to belong to the same super-part, resulting in the similar predicted poses. This highlights that simply relying on geometric similarity to define part-whole hierarchies may sometimes be unreasonable. 

In future work, we plan to incorporate structural information, such as the connection matrix between parts, to further facilitate the process of part-whole hierarchy message passing. 
% Furthermore, considering that in most cases the predicted poses of super-parts provide valuable insights into the hierarchical structure and assembly process of objects, we are interested in developing models that focus on generating individual 3D parts and use our current work as a conditional generation procedure to complete the generation of 3D shapes from scratch.

\begin{figure}
  \centering
  \includegraphics[width=1.0\columnwidth]{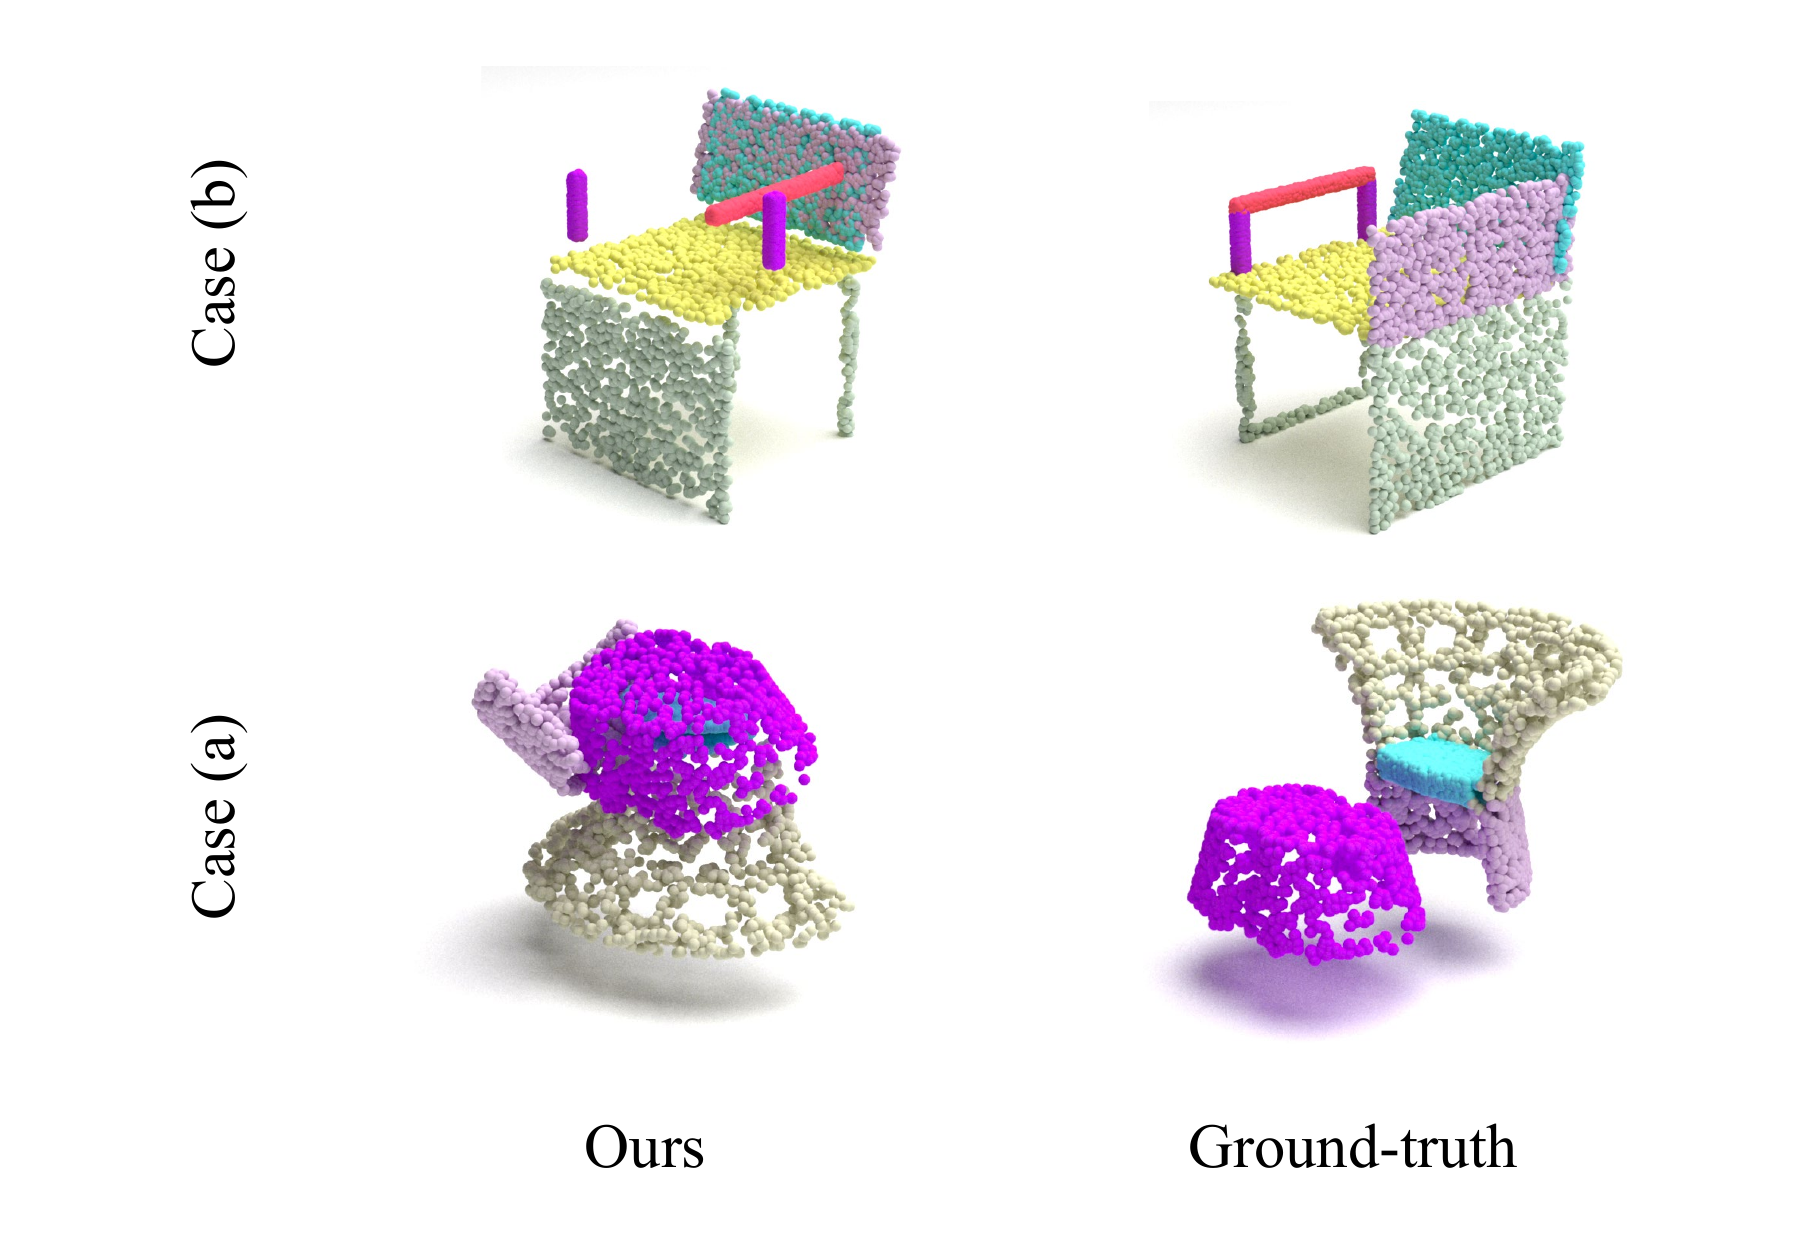}
  \caption{Failure cases where our model fails to assemble shapes effectively.}
  \label{fig:fcfw}
  % \vspace{-0.2in}
\end{figure}

\begin{figure*}
  \centering
  \includegraphics[width=0.85\textwidth]{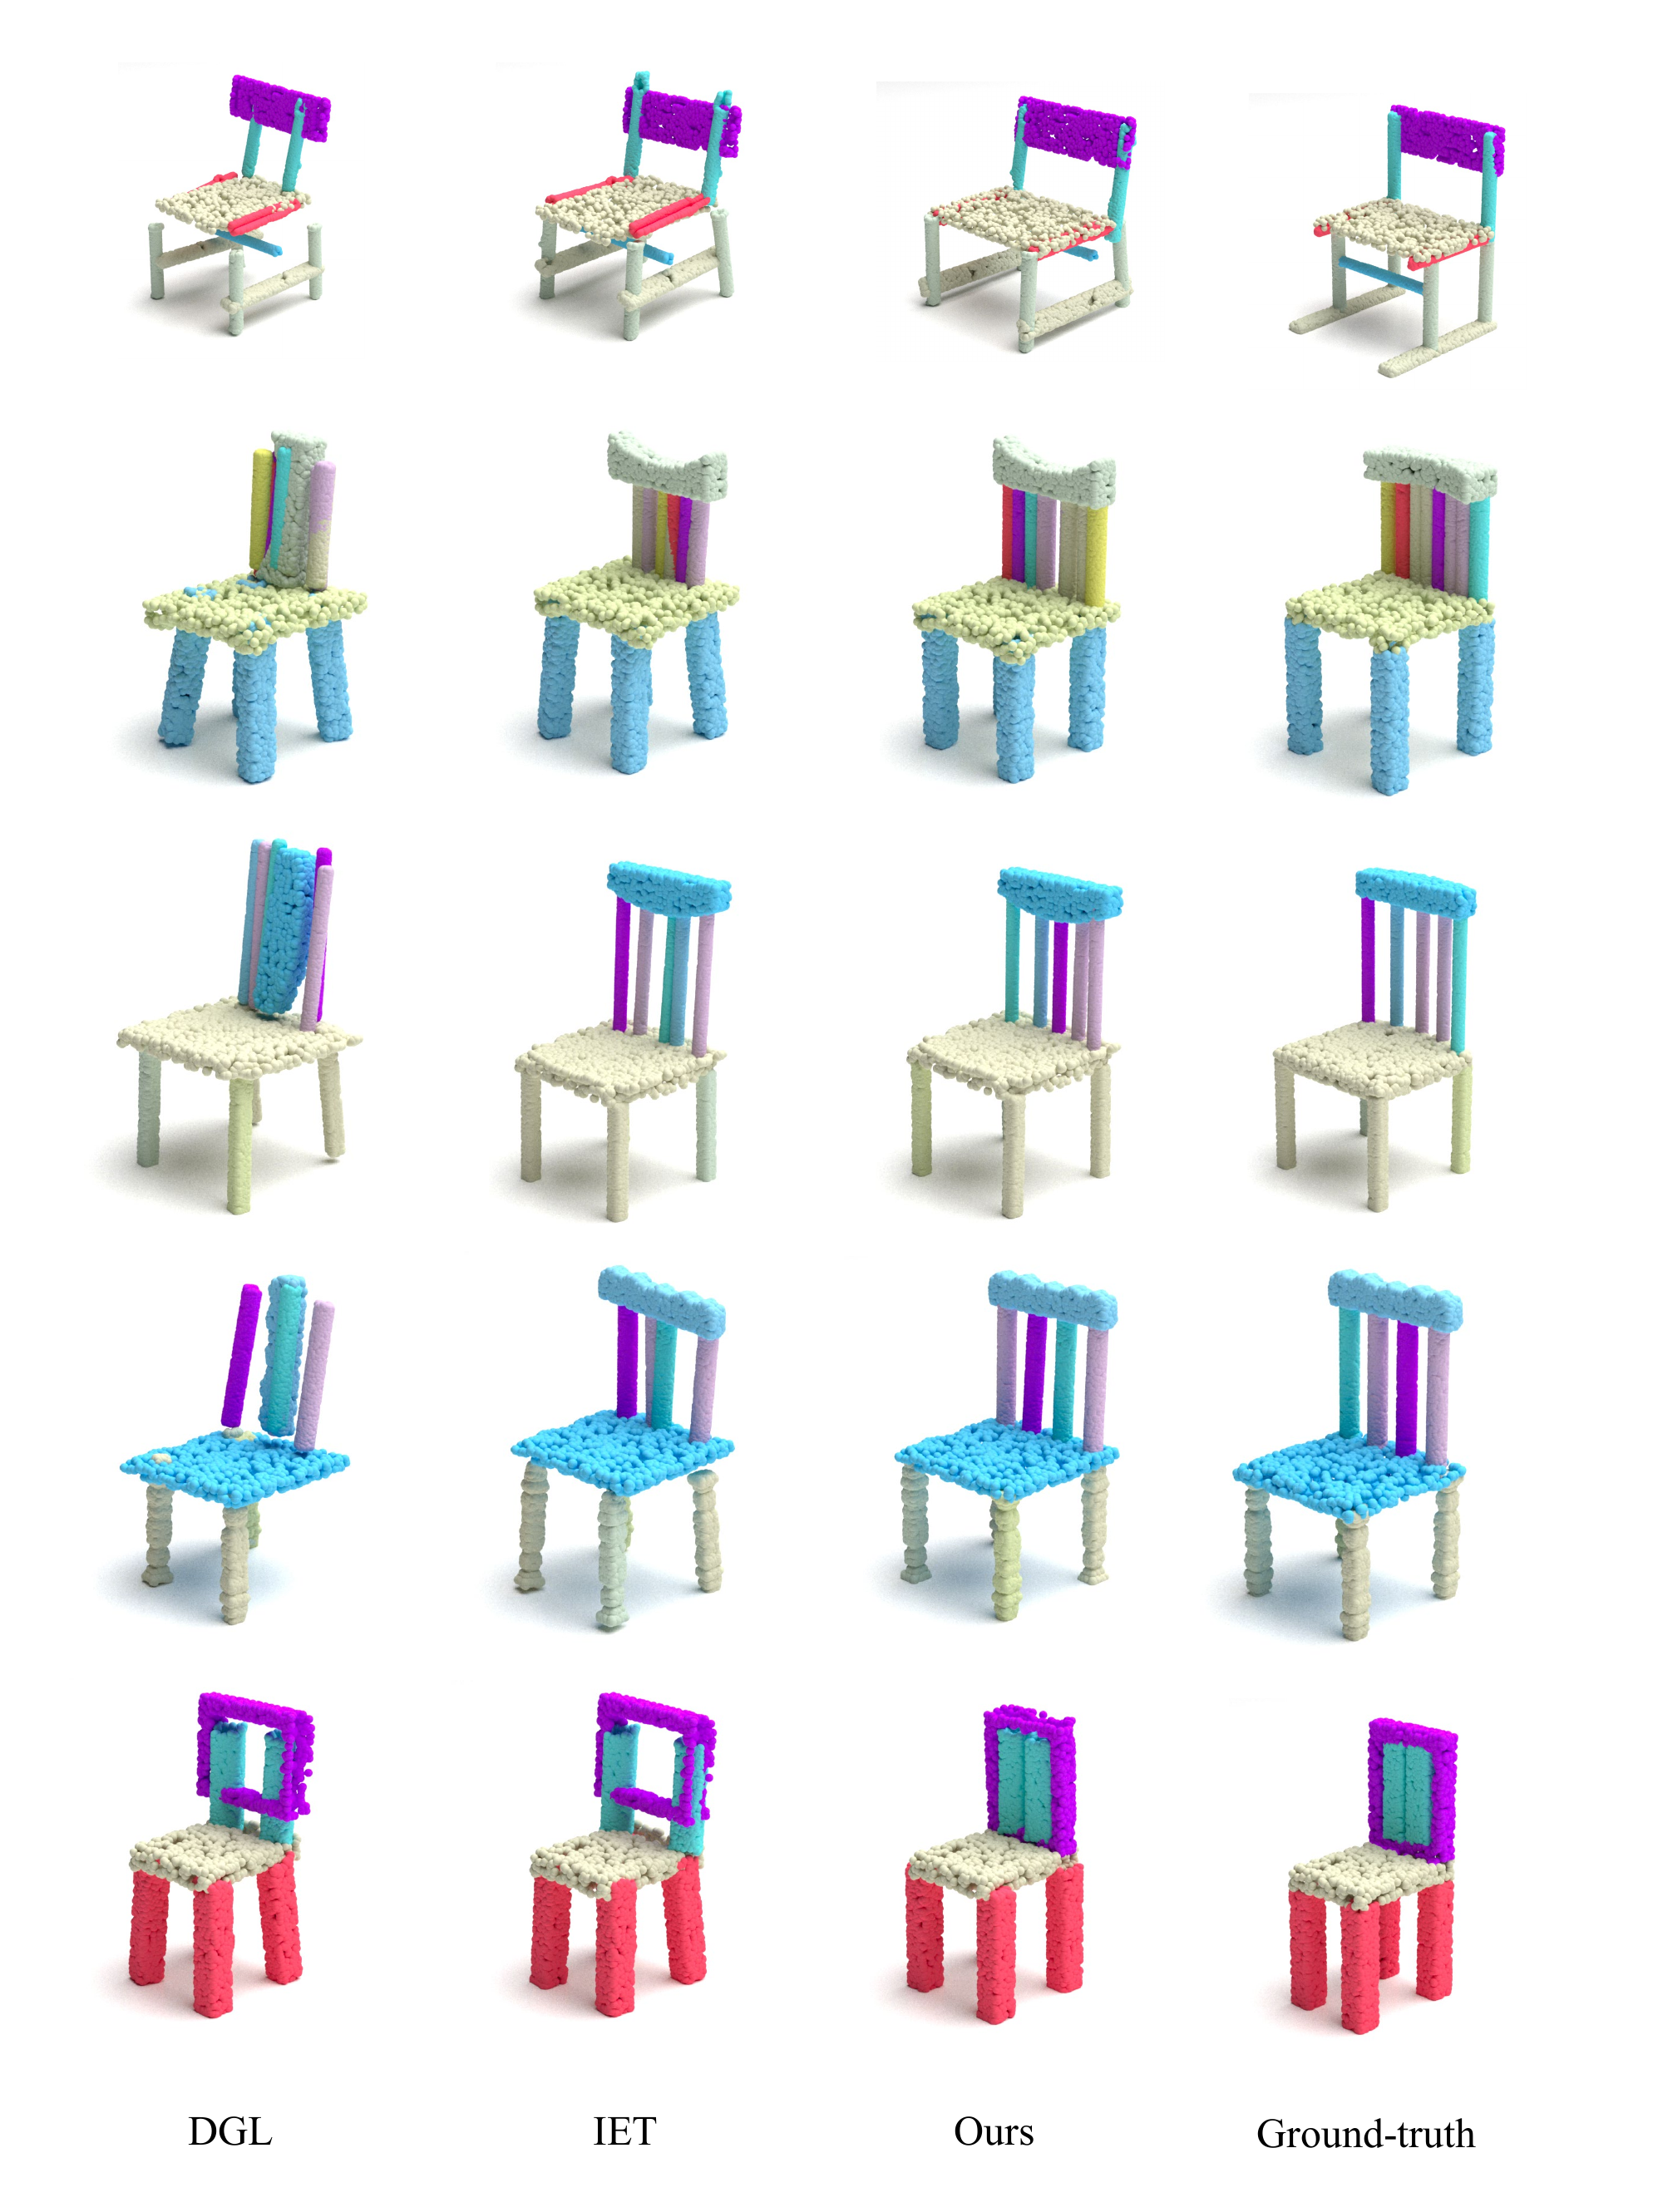}
  \caption{Additional qualitative comparison between our part-whole hierarchy message passing network and other methods on the \textbf{Chair} category.}
  \label{fig:aqr}
  % \vspace{-0.2in}
\end{figure*}

\begin{figure*}
  \centering
  \includegraphics[width=0.9\textwidth]{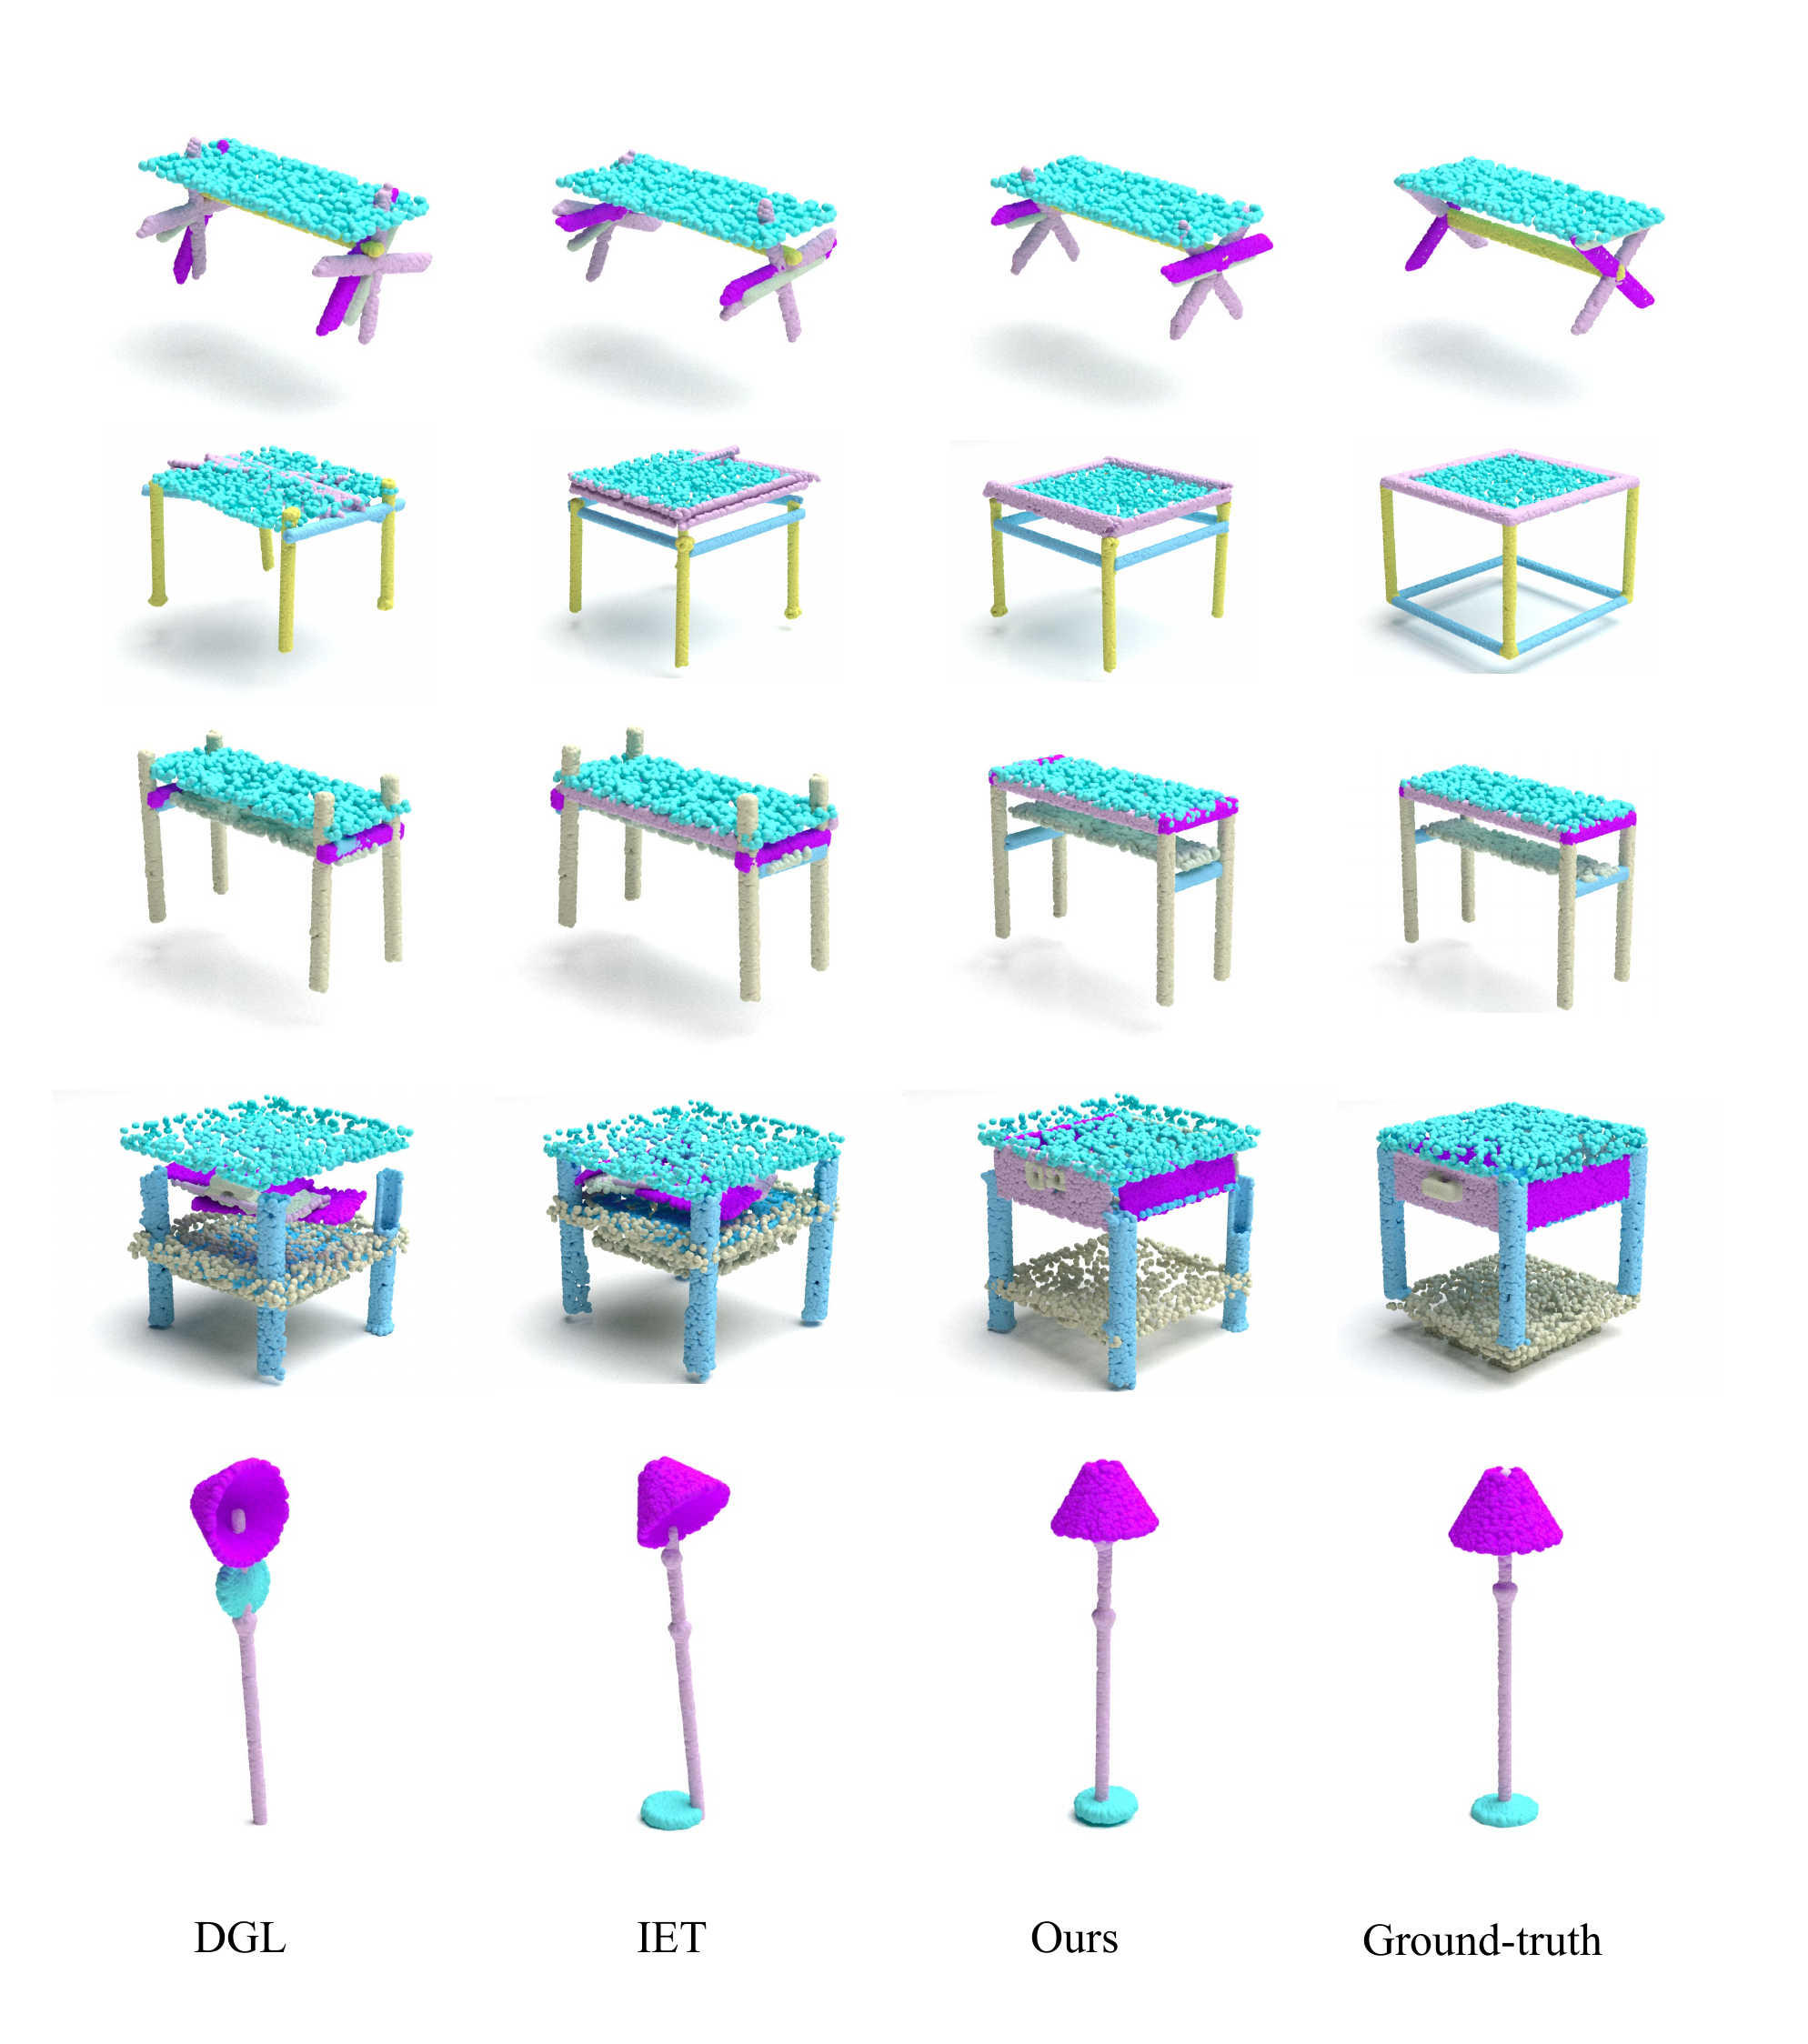}
  \caption{Additional qualitative comparison between our part-whole hierarchy message passing network and other methods on the \textbf{Table} and \textbf{Lamp} category.}
  \label{fig:aqr2}
  % \vspace{-0.2in}
\end{figure*}
